# Supplementary material for: Towards Reproducibility in Predictive Process Mining: SPICE -- A Deep Learning Library
Source: arXiv:2512.16715 source file (2026-08-25)
Supplement: Supplementary file 1 [file appendix.tex]

\begin{table}[]
    \begin{tabularx}{\textwidth}{p{2cm}|X|X|X|X|X|X}
            \textbf{Dataset} & Cases & Unique Activities & Avg. Case Length & Max Case Length & Avg. Throughput Time (days) & \textbf{Available at} \\ \hline 
            BPI 2012 & 13087 & 24 & 20.04 & 175 & 8.62 & \href{https://data.4tu.nl/articles/_/12689204/1}{data.4tu.nl} \\ \hline
            BPI 2013 & 7554 & 4 & 8.68 & 123 & 12.08 & \href{https://data.4tu.nl/articles/_/12693914/1}{data.4tu.nl}  \\ \hline
            BPI 2014 & 46616 & 39 & 10.01 & 178 & 5.07 & \href{https://data.4tu.nl/datasets/657fb1d6-b4c2-4adc-ba48-ed25bf313025/1}{data.4tu.nl}   \\ \hline
            BPI 2015-1 & 1409 & 383 & 42.36 & 124 & 62.23 & \href{https://data.4tu.nl/collections/BPI_Challenge_2015/5065424}{data.4tu.nl} \\ \hline
            BPI 2017 & 31509 & 26 & 38.16 & 180 & 21.90 & \href{https://data.4tu.nl/articles/dataset/BPI_Challenge_2017/12696884}{data.4tu.nl}  \\ \hline
            BPI 2019 & 251734 & 42 & 6.34 & 990 & 71.52 & \href{https://data.4tu.nl/datasets/35ed7122-966a-484e-a0e1-749b64e3366d/1}{data.4tu.nl}  \\ \hline
            BPI 2020d & 10500 & 17 & 5.37 & 24 & 11.53 & \href{https://www.tf-pm.org/competitions-awards/bpi-challenge/2020}{www.tf-pm.org}  \\ \hline
            BPI 2020i & 6449 & 34 & 11.19 & 27 & 86.46 & \href{https://www.tf-pm.org/competitions-awards/bpi-challenge/2020}{www.tf-pm.org}  \\ \hline
            Helpdesk & 4580 & 14 & 4.66 & 15 & 40.86 & \href{https://data.4tu.nl/articles/_/12675977}{data.4tu.nl}  \\ \hline
            Hospital Billing & 99999 & 18 & 4.51 & 217 & 127.36 & \href{https://data.4tu.nl/articles/_/12705113}{data.4tu.nl}  \\ \hline
            Road Traffic & 150370 & 11 & 3.73 & 20 & 341.67 & \href{https://data.4tu.nl/articles/dataset/Road_Traffic_Fine_Management_Process/12683249}{data.4tu.nl}  \\ \hline
    \end{tabularx}
    \caption{Implemented Datasets.}
    \label{tab:benchmark_ds}
\end{table}


\begin{table}[h]
\centering
\begin{tabular}{p{6cm}|c|c}
& & \textbf{Included in}  \\
\textbf{Target} & \textbf{Prediction Method}  & \textbf{initial release} \\
\hline
 Next Activity    &    single-step   & \ding{51} \\
 \hline
 Next Activity     &   multi-step   & \ding{51} \\
 \hline
 Next Timestamp   &    single-step   & \ding{51} \\
 \hline
 Next Timestamp    &   multi-step   & \ding{51} \\
 \hline
 Suffix (Activities/Attributes)   &  iterative \& single-step   & \ding{51} \\
 \hline
 Suffix (Activities/Attributes) &  iterative \& multi-step & \ding{51} \\
 \hline
 Suffix (Timestamps) &  iterative \& single-step  & \ding{51}  \\
 \hline
 Suffix (Timestamps)  &  iterative \& multi-step & \ding{51}  \\
 \hline
 Remaining Time   &   direct    & \ding{51} \\
 \hline
 Remaining Time   &   iterative    & -- \\
 \hline
 Outcome   &   direct    & -- \\
 \hline
 Outcome   &   iterative   & -- \\
\end{tabular}
\caption{Overview of predictive capabilities in our framework. (\ding{51}: supported; --: currently not supported.)}
\label{tab:capabilities}
\end{table}
